# Supplementary material for: BiomedJourney: Counterfactual Biomedical Image Generation by Instruction-Learning from Multimodal Patient Journeys
Source: arXiv:2310.10765 source file (2023-10-21)
Supplement: Supplementary file 1 [file appendix.tex]

% radiologist language severity
\begin{figure}[t]
\begin{minipage}{0.5\linewidth}
\includegraphics[width=.3\textwidth]{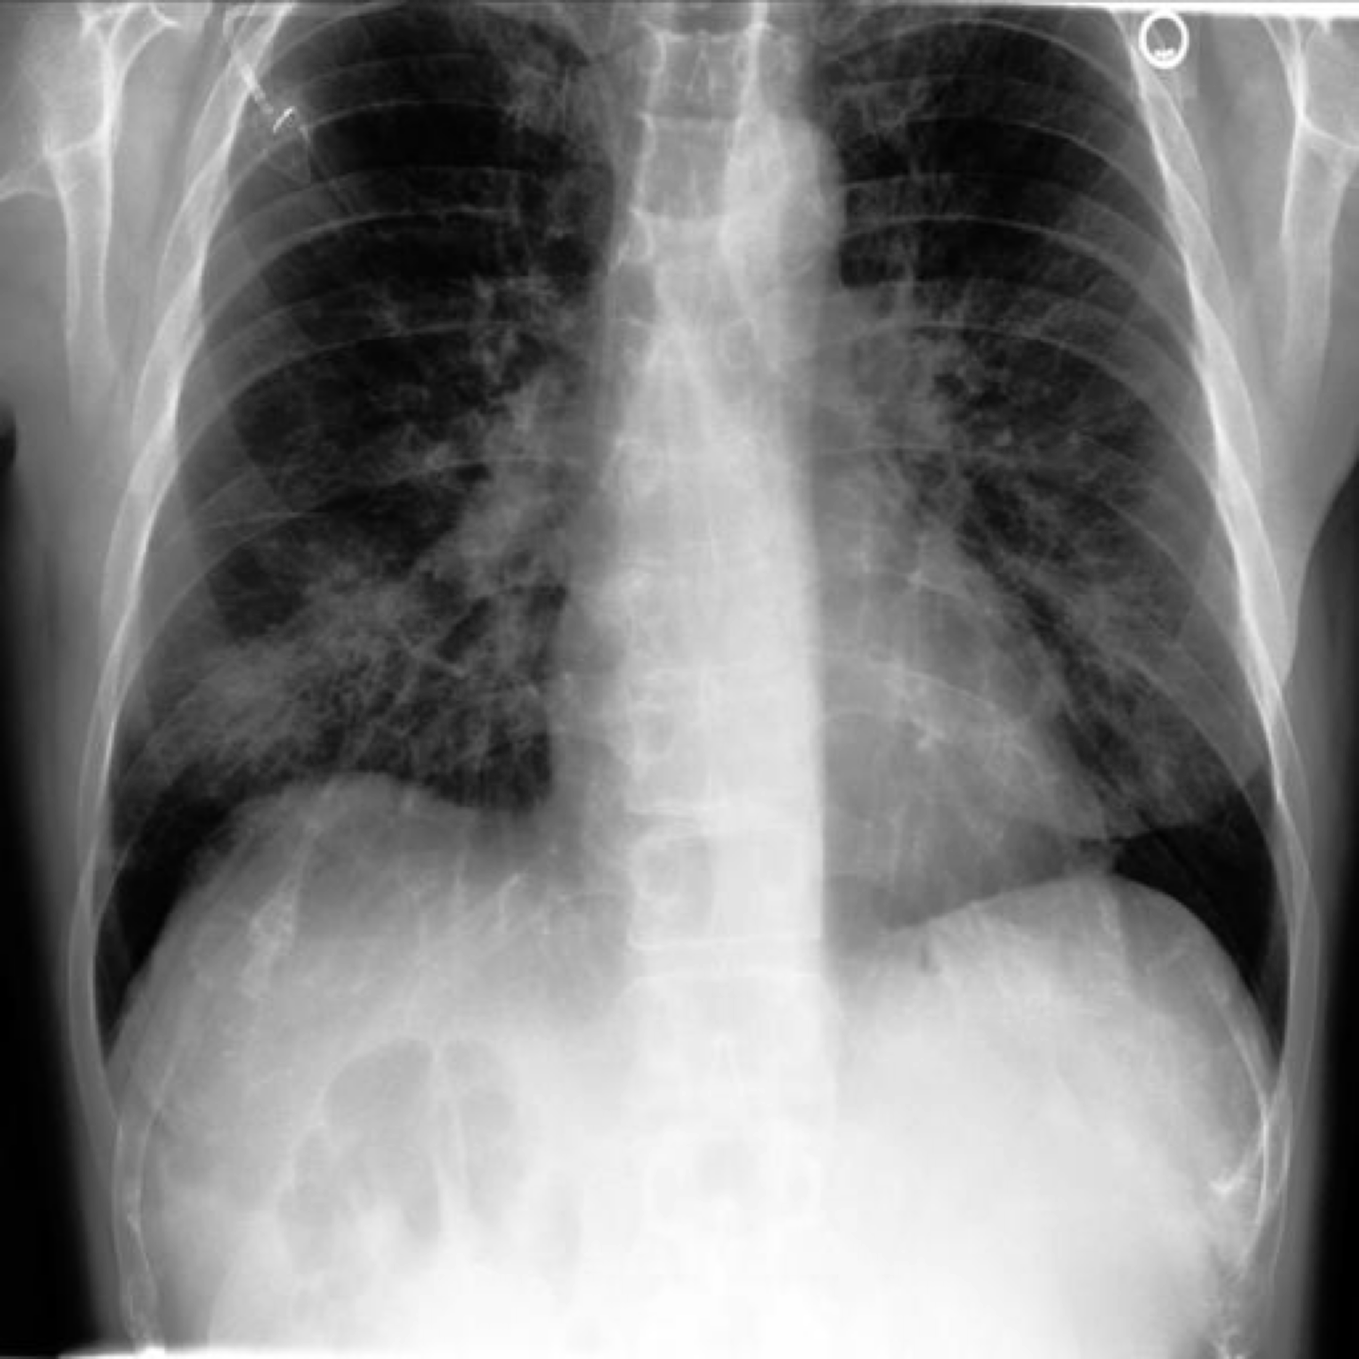}
\includegraphics[width=0.3\textwidth]{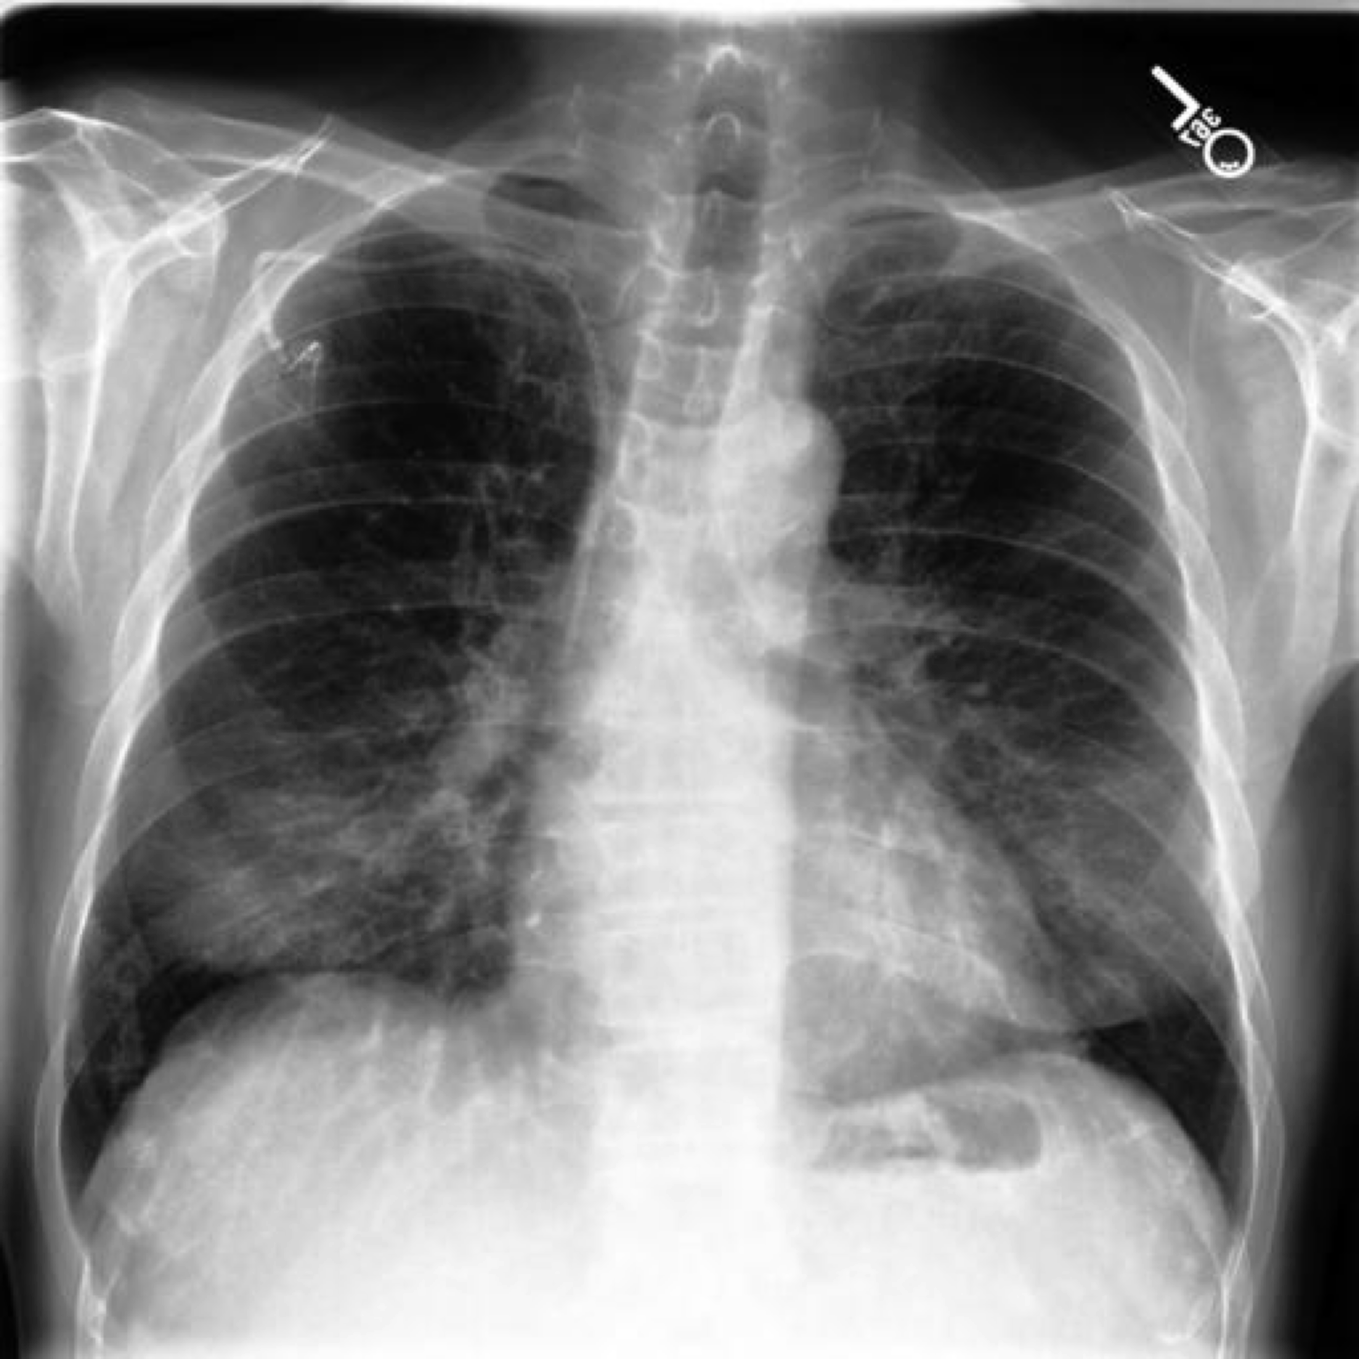}
\includegraphics[width=0.3\textwidth]{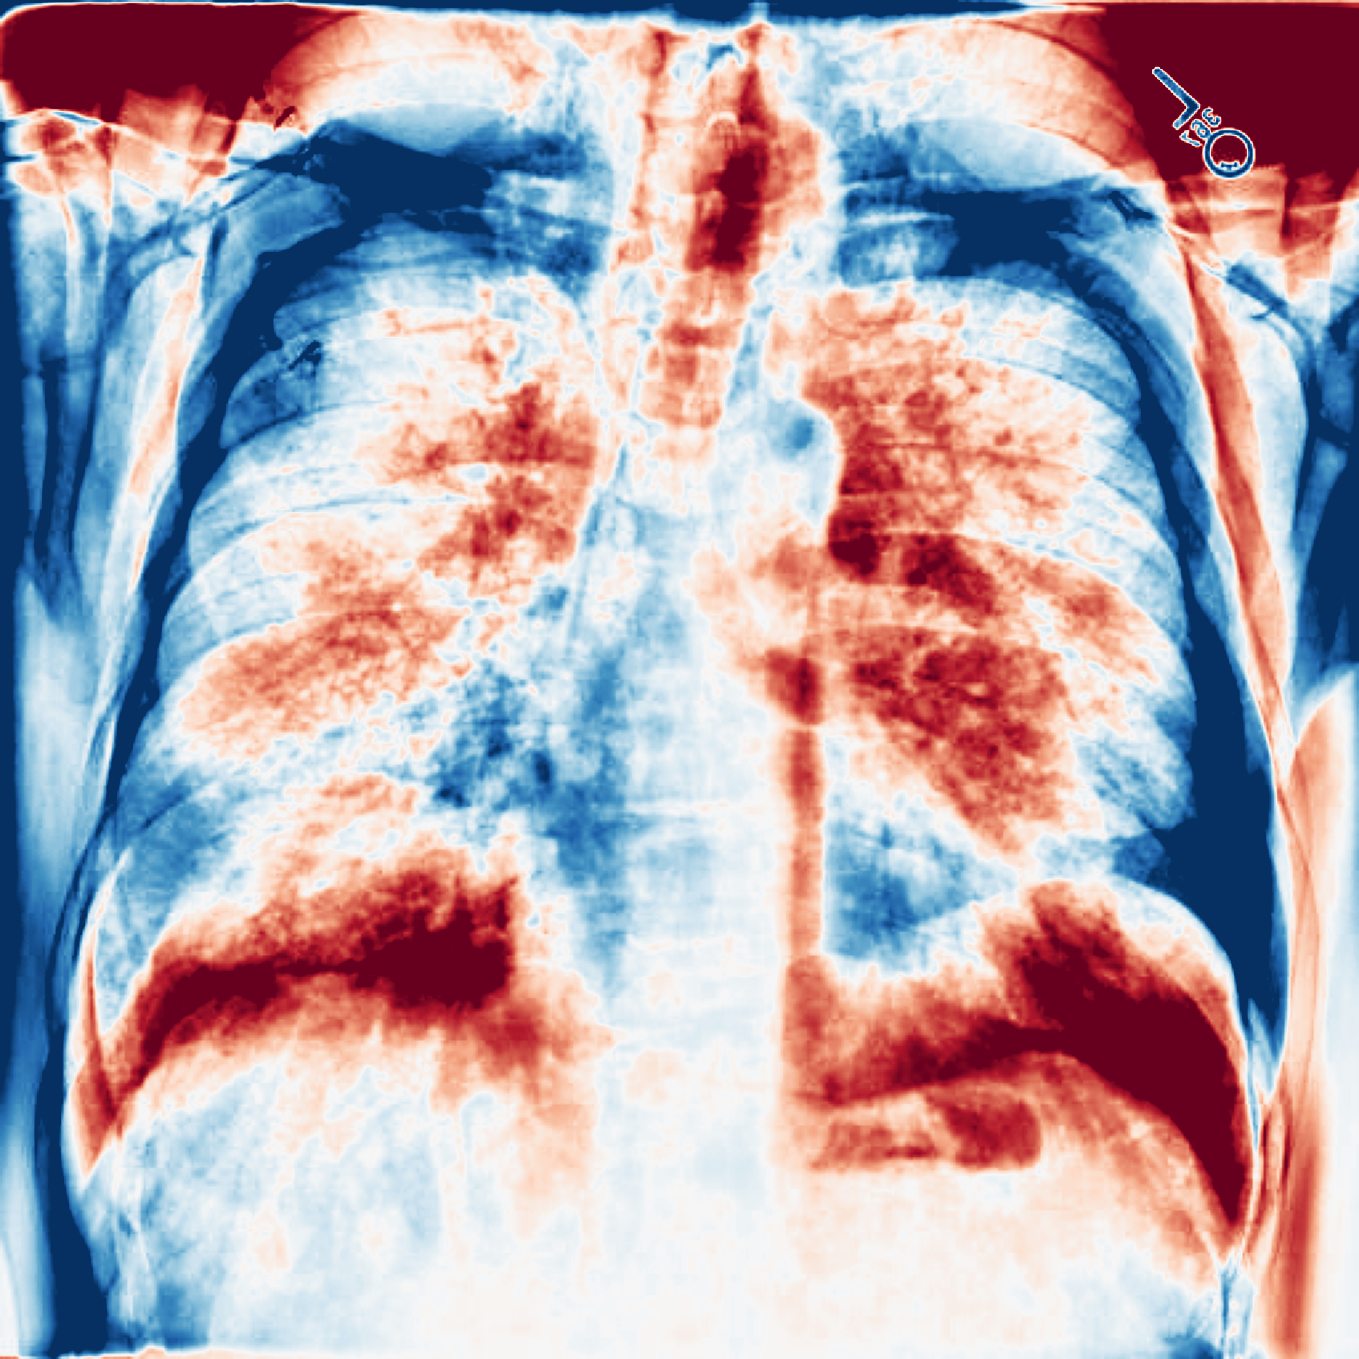}
\end{minipage}
\begin{minipage}{0.5\linewidth}
\includegraphics[width=0.3\textwidth]{figs/registration/Source.png}
\includegraphics[width=0.3\textwidth]{figs/registration/Registered Target.png}
\includegraphics[width=0.3\textwidth]{figs/registration/Post Registration Difference.png}
\end{minipage}
%\framebox[4.0in]{$\;$}
% \includegraphics[width=4.0in]{figs/registration_fig.png}
\caption{Comparison of the target images before and after registration. The left three columns show the source image, the original target image and their difference heatmap; The right three columns show how the registration can help to spatially align the original target image with the source image.\aiden{move to  appendix}}
\label{fig:registraton}
\end{figure}

\section{Conclusion}

We propose \ourmodel, a novel method for counterfactual medical image generation.
